# Supplementary material for: Fun with Flags: Robust Principal Directions via Flag Manifolds
Source: arXiv:2401.04071 source file (2024-08-04)
Supplement: Supplementary file 1 [file appendix_old.tex]

\section{Flagified PCA Variants}
\begin{prop}\label{prop:IRLSPCA}
    Suppose $[\![\Y]\!] \in \flag(n+1)$ solves~\cref{eq: flagRPCAmax} and $\| \Y_i^T \x_j\|_2 \geq \epsilon$ for all $i$ and $j$. Then $\Y \in St(n_k,n)$ must also solve
    \begin{equation}\label{eq:STrealflagPCA}
        \argmax_{\Y \in St(n_k,n)} \tr \left( \A([\![\Y]\!]) \Y \right)
    \end{equation}
    where $\A$ is defined in~\cref{eq:A} using the appropriate weight matrix.
\end{prop}

\begin{proof}
    First, we will translate~\cref{eq: flagRPCAmax} into a problem over $St(n_k,n)$. We begin by defining the matrices
    \begin{equation}\label{eq: Ii}
        (\I_i)_{l,s} = 
        \begin{cases}
            1, & l = s \in \{ n_{j-1} + 1, 
     n_{j-1} + 2, \dots, n_j\} \\
            0, &\text{ otherwise}\nonumber \\
        \end{cases}, 
    \end{equation}
    \begin{equation}\label{eq: Jj}
        \text{and }(\mathbf{J}_j)_{l,s} = 
        \begin{cases}
            1, & l = s = j \\
            0, &\text{ otherwise}\nonumber \\
        \end{cases}.
    \end{equation}
    This allows us to rephrase the optimization problem in~\cref{eq:realflagPCA} as
    \begin{equation}
        \argmax_{\Y \in St(n_k,n)} \sum_{j=1}^p \sum_{i=1}^k \sqrt{\tr\left( \widetilde{\X} \mathbf{J}_j \widetilde{\X}^T \Y \I_i \Y \right)}.
    \end{equation}

    Now, we can write the Lagrangian for this problem with the symmetric matrix of Lagrange multipliers $\bm{\Lambda}$ as
    \begin{equation}
        \mathcal{L} (\Y) = \sum_{j=1}^p \sum_{i=1}^k \sqrt{\tr\left( \widetilde{\X} \mathbf{J}_j \widetilde{\X}^T \Y \I_i \Y \right)} + \bm{\Lambda}(\I - \Y^T \Y ).
    \end{equation}

    Then, we collect our gradients in the following equations
    \begin{align*}
    \begin{aligned}%\label{eq: lagrangian grad}
        \nabla_{\Y} \mathcal{L}
        &=  \sum_{j=1}^p \sum_{i=1}^k \frac{\widetilde{\X} \mathbf{J}_j \widetilde{\X}^T \Y \I_i}{\sqrt{\tr \left( \widetilde{\X} \mathbf{J}_j \widetilde{\X}^T \Y \I_i \Y \right)}} - \bm{\Lambda} \Y\\
         \nabla_{\bm{\Lambda}} \mathcal{L} &=  \I - \Y^T \Y.
    \end{aligned}
    \end{align*}

    With some algebraic manipulation along with the definition of $\mathbf{A}$, we can use $\nabla \mathcal{L} = 0$ to arrive at

    \begin{equation}
        \tr(\bm{\Lambda}) \propto \tr \left( \A([\![\Y]\!]) \Y \right).
    \end{equation}

    Finally we notice that maximizing $\tr(\bm{\Lambda})$ will maximize~\cref{eq:realflagPCA}.

    \nate{The final steps in this proof need some polishing.}
    
\end{proof}


\begin{prop}
    Suppose $[\![\Y]\!] \in \flag(n+1)$ solves~\cref{eq: flagRPCAmin} and $\| \Y_i^T \x_j\|_2 \geq \epsilon$ for all $i$ and $j$. Then $\Y \in St(n_k,n)$ must also solve
    \begin{equation}\label{eq:STrealflagPCA}
        \argmin_{\Y \in St(n_k,n)} \tr \left( \A([\![\Y]\!]) \Y \right)
    \end{equation}
    where $\A$ is defined in~\cref{eq:A} and $\W_i$ is defined using~\cref{eq: min_weights}.
\end{prop}

\begin{prop}
    Suppose $[\![\Y]\!] \in \flag(n+1)$ solves~\cref{eq: flagDPCAmax} and $\| \Y_i^T \x_j\|_2 \geq \epsilon$ for all $i$ and $j$. Then $\Y \in St(n_k,n)$ must also solve
    \begin{equation}\label{eq:STrealflagPCA}
        \argmin_{\Y \in St(n_k,n)} \tr \left( \A([\![\Y]\!]) \Y \right)
    \end{equation}
    where $\A$ is defined in~\cref{eq:A} and $\W_i$ is defined using~\cref{eq: min_weights}.
\end{prop}

\begin{prop}
    Suppose $[\![\Y]\!] \in \flag(n+1)$ solves~\cref{eq: flagDPCAmin} and $\| \Y_i^T \x_j\|_2 \geq \epsilon$ for all $i$ and $j$. Then $\Y \in St(n_k,n)$ must also solve
    \begin{equation}\label{eq:STrealflagPCA}
        \argmax_{\Y \in St(n_k,n)} \tr \left( \A([\![\Y]\!]) \Y \right)
    \end{equation}
    where $\A$ is defined in~\cref{eq:A} and $\W_i$ is defined using~\cref{eq: min_weights}.
\end{prop}


\section{DPCP-IRLS and the Grassmannian}\label{sec:grassdpcp}
Expanding the matrix norm we have
\begin{align}
    \| \X^T \B \|_{1,2} &= \sum_{j=1}^p \| \B^T \x_j \|_2,\\
    &= \sum_{j=1}^p \sqrt{\sum_{i=1}^k | \vb_i^T \x_j|^2 }, \\
    &= \sum_{j=1}^p \sqrt{ \x_j^T \B \B^T \x_j }, \\
    &= \sum_{j=1}^p \sqrt{ \tr\left( \B^T \x_j  \x_j^T \B \right) }.
\end{align}
This can be phrased using principal angles as
\begin{equation}
    \argmin_{\B^T \B = \I} \sum_{j=1}^p \cos \theta([\x_j], [\B]).
\end{equation}
% which is equivalent to
% \begin{equation}
%     \argmax_{\B^T \B = \I} \sum_{j=1}^p \sin \theta([\x_j], [\B]).
% \end{equation}
Suppose $\{[\X_j]\}_{j=1}^p \subset \Gr(k,n)$. Namely, $\X_j \in \R^{n \times k}$ where $\X_j^T \X_j = \I$ for each $j$. A natural generalization of DPCP-IRLS is the optimization problem on the Grassmannian,
\begin{equation}\label{eq:grassdpcp}
    \argmin_{[\B]\in \Gr(k,n)} \sum_{j=1}^p \| \cos \theta([\X_j], [\B])\|_2.
\end{equation}
This can also be solved by an IRLS scheme.

The ``flagified'' version of~\cref{eq:grassdpcp} is
\begin{equation}
    \argmin_{[\![ \B ]\!] \in \flag(n+1)} \sum_{j=1}^p \| \cos \theta([\X_j], [\B])\|_2.
\end{equation}

\section{Manifold Means}\label{sec:manmeans}
\textcolor{blue}{WRITE THIS SECTION}


\section{Proofs}
\subsection{PCA}
\begin{prop}\label{prop: pcaexp}
Define $S_i  = \text{span} (  \mathbf{u}_1, \mathbf{u}_2, \dots, \mathbf{u}_i)$ and  $S_{\mathbf{u}}  = \text{span} \left(  S_{i-1} \cup \{\mathbf{u} \}\right)$. The $i$th principal component is
\begin{equation}\label{eq: generalpca}
\mathbf{u}_{i} = \argmax_{\substack{\mathbf{u}^T \mathbf{u} = 1 \\ \mathbf{u} \in S_{i-1}^\perp}} \mathbb{E} \left[ \|  \bm{\mu} - \pi_{S_{\mathbf{u}}} (\x_j) \|^q \right]
\end{equation}
for $q=2$.
\end{prop}


\begin{proof}
Let $\mathbf{U}_i = [\mathbf{u}_1, \mathbf{u}_2, \dots, \mathbf{u}_i, \mathbf{u}]$. Then we compute the expected value
\begin{align}
&\mathbb{E} \left[ \|  \bm{\mu} - \pi_{S_\mathbf{u}} (\x_j) \|^2 \right],\\
&=\sum_{j=1}^p \|  \bm{\mu} - \pi_{S_\mathbf{u}} (\x_j) \|^2, \\
&= \sum_{j=1}^p \|  \bm{\mu} -  \mathbf{U}_i \mathbf{U}_i^T \x_j \|^2, \\
&= \sum_{j=1}^p \x_j^T\mathbf{U}_i \mathbf{U}_i^T \x_j  - 2\bm{\mu}^T \mathbf{U}_i \mathbf{U}_i^T  \x_j + \bm{\mu}^T \bm{\mu}.
\end{align}
Notice $\bm{\mu}^T \bm{\mu}$ is constant with respect to $\mathbf{
u}$. So maximizing the expression above is equivalent to maximizing
\begin{align}
&\sum_{j=1}^p \x_j^T\mathbf{U}_i \mathbf{U}_i^T \x_j  - 2\bm{\mu}^T \mathbf{U}_i \mathbf{U}_i^T  \x_j,\\
&=\sum_{j=1}^p -\bm{\mu}^T \mathbf{U}_i \mathbf{U}_i^T  \x_j + \x_j^T\mathbf{U}_i \mathbf{U}_i^T \x_j  - \x_j \mathbf{U}_i \mathbf{U}_i^T  \bm{\mu}^T,\\
&=\sum_{j=1}^p(\x_j - \bm{\mu}) ^T\mathbf{U}_i \mathbf{U}_i^T(\x_j - \bm{\mu}),\\
&=\tr \left( \mathbf{U}_i^T \left( \sum_{j=1}^p(\x_j - \bm{\mu}) (\x_j - \bm{\mu})^T \right) \mathbf{U}_i\right),\\
&=\tr \left( \mathbf{U}_i^T \widetilde{\X} \widetilde{\X}^T \mathbf{U}_i\right).
\end{align}
So finding the directions of maximum variance is equivalent to PCA.
\end{proof}

%\begin{align}
%&\sum_{j=1}^p \x_j^T\mathbf{U}_i \mathbf{U}_i^T \x_j  - 2\bm{\mu}^T \mathbf{U}_i \mathbf{U}_i^T  \x_j \\
%&= \sum_{j=1}^p \x_j^T\mathbf{U}_i \mathbf{U}_i^T \x_j  - 2\bm{\mu}^T \mathbf{U}_i \mathbf{U}_i^T  \x_j 
%\end{align}
%So, this is equivalent to INSERT TANGENT PGA NOTATION.


%\begin{align}
%&\sum_{j=1}^n \x_j^T \mathbf{u}_i \mathbf{u}_i^T \x_j  - 2\bm{\mu}^T \mathbf{u}_i \mathbf{u}_i^T \x_j \\
%&=\tr \left( \mathbf{u}_i^T \left( \sum_{j=1}^n \x_j^T \x_j  - 2\bm{\mu}^T  \x_j \right) \mathbf{u}_i^T \right) \\
%&=\tr \left( \mathbf{u}_i^T \left( \sum_{j=1}^n  -\x_j^T\bm{\mu}   \x_j^T \x_j  - \bm{\mu}^T  \x_j \right) \mathbf{u}_i^T \right) \\
%&=\tr \left( \mathbf{u}_i^T \left( \sum_{j=1}^n (\x_j-\bm{\mu})^T (\x_j  - \bm{\mu})^T \right) \mathbf{u}_i^T \right) 
%\end{align}


\begin{prop}
    Suppose $\{w_j\}_{j=1}^p \subset \R^n$ is a mean centered dataset. Then the $i$th principal component of this dataset is
    \begin{equation}
        u_{i} =\argmax_{\substack{ \| u \| = 1 \\ u \in S_i^\perp}}  \sum_{j=1}^p \left( \langle w_j, u \rangle^2 + \sum_{l=1}^{i-1} \langle w_j, u_l \rangle^2 \right).
    \end{equation}
\end{prop}
\begin{proof}
    Take $\{u\}, \{u_l\}_{l=1}^{i-1}, \{w_j\}_{j=1}^p \subset \R^n$ and $\langle \cdot, \cdot \rangle$ as the standard inner product. Let $\U_i = [\mathbf{u}_1, \mathbf{u}_2, \dots, \mathbf{u}_{i-1}, \mathbf{u}]$ and $\mathbf{W} = [\mathbf{w}_1,\mathbf{w}_2,\dots, \mathbf{w}_p]$. Then we re-arrange the objective function:
    \begin{align}
        &\sum_{j=1}^p \left( \langle \mathbf{w}_j, \mathbf{u} \rangle^2 + \sum_{l=1}^{i-1} \langle \mathbf{w}_j, \mathbf{u}_l \rangle^2 \right), \\
        &= \sum_{j=1}^p \langle \mathbf{w}_j, \mathbf{u} \rangle^2 + \sum_{l=1}^{i-1} \sum_{j=1}^p\langle \mathbf{w}_j, \mathbf{u}_l \rangle^2,\\
        &= \sum_{j=1}^p \langle \mathbf{w}_j, \mathbf{u} \rangle^2 + \sum_{l=1}^{i-1} \sum_{j=1}^p \mathbf{u}_l^T \mathbf{w}_j^T \mathbf{w}_j \mathbf{u}_l,\\
        &= \sum_{j=1}^p \mathbf{u}^T \mathbf{w}_j \mathbf{w}_j^T u + \sum_{l=1}^{i-1} \mathbf{u}_l^T \left( \sum_{j=1}^p  \mathbf{w}_j^T \mathbf{w}_j \right) \mathbf{u}_l,\\
        &= \mathbf{u}^T \left( \sum_{j=1}^p  \mathbf{w}_j \mathbf{w}_j^T \right)  \mathbf{u}  + \sum_{l=1}^{i-1} \mathbf{u}_l^T \left( \sum_{j=1}^p  \mathbf{w}_j^T \mathbf{w}_j \right) u_l,\\
        &= \mathbf{u}^T \left( \sum_{j=1}^p  \mathbf{w}_j \mathbf{w}_j^T \right)  \mathbf{u}  + \sum_{l=1}^{i-1} \mathbf{u}_l^T \left( \sum_{j=1}^p  \mathbf{w}_j^T \mathbf{w}_j \right) \mathbf{u}_l,\\
        % &= \tr \left( [u_1, \dots, u_{i-1}, u]^T \left( \sum_{j=1}^p  w_j w_j^T \right)  [u_1, \dots, u_{i-1}, u]\right),\\
        &= \tr \left( \U_i^T \mathbf{W}^T  \mathbf{W}  \U_i\right).
    \end{align}
    So $\mathbf{u}_1, \mathbf{u}_2, \dots,  \mathbf{u}_k$ can be found simultaneously by solving
    \begin{equation}
        \U = \argmax_{\Y^T \Y = \I} \tr(\Y^T \W \W^T \Y).
    \end{equation}
\end{proof}


\subsection{Dual PCA}
\begin{prop}
    Let $\{\x_i\}_{i=1}^p \subset \R^n$ and define $\hat{\x}_i =  \x_i / \| \x_i \|$. DPCP is equivalent to
    \begin{equation}
        b_{i} = \argmin_{\substack{ \| b \| = 1 \\ b \in S_{i-1}^\perp}}  \mathbb{E} \left[ \langle  \x_i, \pi_{S_b} (\x_i) \rangle^{1/2} \right].
    \end{equation}
\end{prop}
\begin{proof}
     Take some unit vector $\vb \in \R^n$. Then the objective function of DPCP is
    \begin{align}
        \|\X^T \vb\| &= \sum_{j=1}^p |\x_j^T \vb|,\\
        &= \sum_{j=1}^p \sqrt{(\x_j^T \vb)^2}, \\
        &= \sum_{j=1}^p \sqrt{\x_j^T \vb \vb^T\x_j }, \\
        &= \sum_{j=1}^p \sqrt{\x_j^T \pi_{S_b} (\x_j) }, \\
        &= \sum_{j=1}^p\sqrt{\langle  \x_j, \pi_{S_b} (\x_i) \rangle}, \\
        &= p \: \mathbb{E} \left[ \langle  \x_j, \pi_{S_b} (\x_i) \rangle^{1/2} \right].
    \end{align}
    So, minimizing $\|\X^T \vb\|$ is the same as minimizing $\mathbb{E} \left[ \langle  \x_j, \pi_{S_b} (\x_i) \rangle^{1/2} \right].$
\end{proof}



\section{Examples}

\subsection{Flagified PCA}
Suppose we sample points $\{\x^{(i)}\}_{i=1}^{5000} \subset \R^4$ with coordinates sampled as $\x^{(i)}_1, \x^{(i)}_2 \sim \mathcal{N}(0,1)$, $\x^{(i)}_3 \sim \mathcal{N}(0,0.5)$, and $\x^{(i)}_4 \sim \mathcal{N}(0,0.1)$ where $\mathcal{N}(\mu,\sigma)$ is a normal distribution with mean $\mu$ and standard deviation $\sigma$. PCA on these data is in~\cref{fig:why_flag_pca0},~\cref{fig:why_flag_pca1},~\cref{fig:why_flag_pca2}, and~\cref{fig:why_flag_pca3}. Notice that we should preform PCA on $\flag(2,3,4;5)$ instead of $\flag(1,2,3,4;5)$
\begin{figure}[H]
    \centering
    \includegraphics{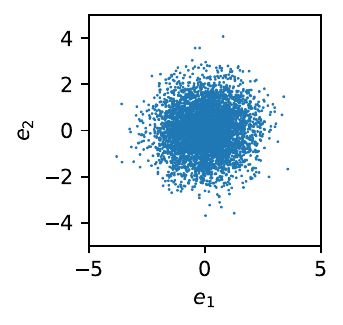}
    \caption{Mapping the data onto $\mathbf{e}_1 = [1,0,0,0]^T$ and $\mathbf{e}_1 = [0,1,0,0]^T$. Any basis vectors orthogonal to $\text{span}(\mathbf{e}_3, \mathbf{e}_4)$ will work for the first two principle components of our data.}
    \label{fig:why_flag_pca0}
\end{figure}

\begin{figure}[H]
    \centering
    \includegraphics{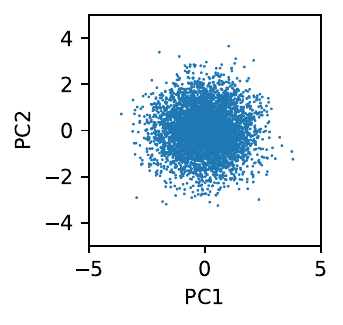}
    \caption{Mapping the data onto the first two principle components. Any basis vectors orthogonal to $\text{span}(\mathbf{e}_3, \mathbf{e}_4)$ will work for the first two principle components of our data.}
    \label{fig:why_flag_pca1}
\end{figure}

\begin{figure}[H]
    \centering
    \includegraphics[width =\linewidth]{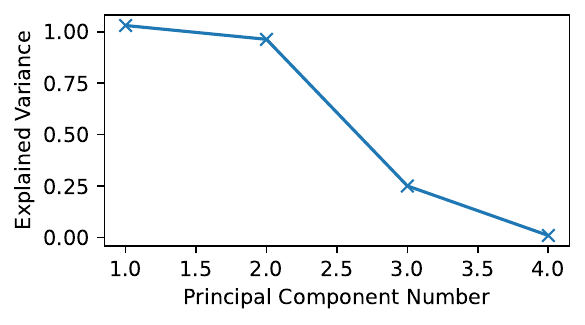}
    \caption{The explained variances (objective function values) for the PCs.}
    \label{fig:why_flag_pca2}
\end{figure}

\begin{figure}[H]
    \centering
    \includegraphics[width =\linewidth]{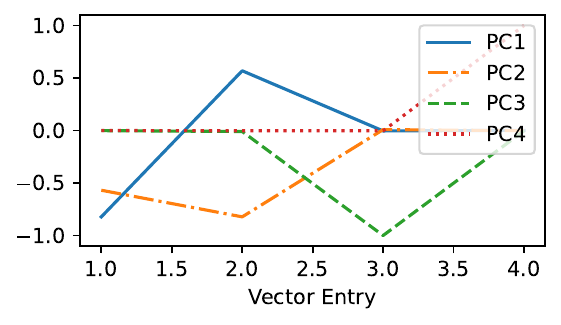}
    \caption{The PCs.}
    \label{fig:why_flag_pca3}
\end{figure}


\subsection{Unorganized}
Suppose we have $p$ samples (points) with $n$ random variables (features) $\mathcal{X} = \{ \x_i \}_{i=1}^p \subset \R^n$. We write the data matrix with samples as columns $\X = [\x_1, \x_2, \dots, \x_p] \in \R^{n\times p}$ The Euclidean mean of our samples is $\mu = \frac{1}{n} \sum_{j=1}^p \x_j$. Using this, our mean-centered samples are $\widetilde{\x}_j = \x_j - \bm{\mu}$ and mean-centered data matrix is $\widetilde{\X} =  [\widetilde{\x}_1 , \widetilde{\x}_2 , \dots, \widetilde{\x}_p ]$ and the sample covariance matrix $\widetilde{\X} \widetilde{\X}^T \in \R^{n \times n}$.


\begin{dfn}[PCA~\cite{hotelling1933analysis}]
The first $k$ \emph{principal components}\footnote{ These are sometimes called the principal component weights or Empirical Orthogonal Functions.} of $\mathcal{X}$ are the columns of
\begin{equation}\label{eq:pca_opt}
\U = \argmax_{\Y^T \Y = \I} \tr(\Y^T \widetilde{\X} \widetilde{\X}^T \Y).
\end{equation}
\end{dfn}
PCA has been kernelized to improve performance when $p << n$ and better represent non-linear structures in data~\cite{scholkopf1997kernel}. In general, PCA gives us a $k<n$ dimensional embedding of the data as the columns of $\U^T\widetilde{\X} \in \R^{k \times p}$. We can approximately invert PCA by left multiplication by $\U$.

\begin{remark}
    The solution for PCA is the first $k$ left singular vectors of $\widetilde{\X}$, or equivalently, the first $k$ eigenvectors of the mean-centered covariance matrix.  It is standard to order the columns of $\U$ according to their associated explained variances (eigenvalues) $\lambda_i = \bu^T \widetilde{\X} \widetilde{\X}^T \bu_i$. Specifically, we order the principal components as $\lambda_{i} \geq \lambda_{i+1}$. But, in~\cref{eq:pca_opt}, there is no restriction on the ordering of the columns of the matrix $\Y$ because
    \begin{equation}
        \tr(\Y^T \widetilde{\X} \widetilde{\X}^T \Y) = \sum_{i=1}^k \y_i^T \widetilde{\X} \widetilde{\X}^T \y_i.
    \end{equation}
    Since the objective function in~\cref{eq:pca_opt} is invariant to ordering the columns of $\Y$, it is an objective function defined over a Grassmannian.
    
    % The PCA objective function is essentially the sum of the first $k$ eigenvalues of the matrix $\widetilde{\X}\widetilde{\X}^T$. This sum is invariant to the permutations of the columns of $\U$ (eigenvectors) because these permutations only change the order of the eigenvalues of the sum and addition is commutative. Therefore, in this formulation, any ordering of the columns of $\U$ produces the same objective function values. \nate{Elaborate on this and formalize mathematically.}
\end{remark}

\paragraph{Formalizing PCA}

% Note: there is no need to distinguish between a geodesic subspace and a subspace of the tangent space. 


\begin{prop}\label{prop: pcaexp}
Define $S_i  = \text{span} (  \mathbf{u}_1, \mathbf{u}_2, \dots, \mathbf{u}_i)$ and  $S_{\mathbf{u}}  = \text{span} \left(  S_{i-1} \cup \{\mathbf{u} \}\right)$. The $i$th principal component is
\begin{equation}\label{eq: generalpca}
\mathbf{u}_{i} = \argmax_{\substack{\mathbf{u}^T \mathbf{u} = 1 \\ \mathbf{u} \in S_{i-1}^\perp}} \mathbb{E} \left[\|  \bm{\mu} - \pi_{S_{\mathbf{u}}} (\x_j) \|^q \right]
\end{equation}
for $q=2$. Set $q=1$ for the $i$th ``robust'' principal component.
\end{prop}
The above definition uses $x^q$ as the function of the distance. We can generally replace $x^q$ with any monotonic function from $\R^+$ to $\R$. Neumayer~\etal~\cite{neumayer2020robust} noted this fact and proposed a provably convergent algorithm for computing robust PCA ($q=1$). Other notions of robust PCA have also been considered~\cite{candes2011robust, vidal2018dpcp}.

\begin{proof}
    See Appendix.
\end{proof}

%\begin{align}
%&\sum_{j=1}^p \x_j^T\mathbf{U}_i \mathbf{U}_i^T \x_j  - 2\bm{\mu}^T \mathbf{U}_i \mathbf{U}_i^T  \x_j \\
%&= \sum_{j=1}^p \x_j^T\mathbf{U}_i \mathbf{U}_i^T \x_j  - 2\bm{\mu}^T \mathbf{U}_i \mathbf{U}_i^T  \x_j 
%\end{align}
%So, this is equivalent to INSERT TANGENT PGA NOTATION.


%\begin{align}
%&\sum_{j=1}^n \x_j^T \mathbf{u}_i \mathbf{u}_i^T \x_j  - 2\bm{\mu}^T \mathbf{u}_i \mathbf{u}_i^T \x_j \\
%&=\tr \left( \mathbf{u}_i^T \left( \sum_{j=1}^n \x_j^T \x_j  - 2\bm{\mu}^T  \x_j \right) \mathbf{u}_i^T \right) \\
%&=\tr \left( \mathbf{u}_i^T \left( \sum_{j=1}^n  -\x_j^T\bm{\mu}   \x_j^T \x_j  - \bm{\mu}^T  \x_j \right) \mathbf{u}_i^T \right) \\
%&=\tr \left( \mathbf{u}_i^T \left( \sum_{j=1}^n (\x_j-\bm{\mu})^T (\x_j  - \bm{\mu})^T \right) \mathbf{u}_i^T \right) 
%\end{align}


\begin{prop}
    Suppose $\{w_j\}_{j=1}^p \subset \R^n$ is a mean centered dataset. Then the $i$th principal component of this dataset is
    \begin{equation}
        u_{i} =\argmax_{\substack{ \| u \| = 1 \\ u \in S_i^\perp}}  \sum_{j=1}^p \left( \langle w_j, u \rangle^2 + \sum_{l=1}^{i-1} \langle w_j, u_l \rangle^2 \right).
    \end{equation}
\end{prop}

\begin{proof}
    See Appendix.
\end{proof}


\section{Old Proofs}

    \nate{No Lagrangians here. Just adapt each of these objective functions to Stiefel objective functions.}

    Now, we can write the Lagrangians for these problems with the symmetric matrix of Lagrange multipliers $\bm{\Lambda}$ as
    \begin{align*}
        \mathcal{L}_1 (\U) &= \sum_{j=1}^p \sum_{i=1}^k \tr \left(\U^T \x_j  \x_j^T \U \I_i\right) + \bm{\Lambda}_1(\I - \U^T \U ),\\
        \mathcal{L}_2 (\U) &= \sum_{j=1}^p \sum_{i=1}^k \tr \left(\x_j^T\x_j - \U^T \x_j  \x_j^T \U \I_i\right)+ \bm{\Lambda}_2(\I - \U^T \U ).
    \end{align*}
    Then, we collect our gradients in the following equations
    \begin{align*}
    \begin{aligned}%\label{eq: lagrangian grad}
        \nabla_{\U} \mathcal{L}_1
        &=  \sum_{j=1}^p \sum_{i=1}^k \frac{\x_j \x_j^T \U \I_i}{\| \U_i^T \x_j\|_2} - \bm{\Lambda}_1 \U\\
         \nabla_{\U} \mathcal{L}_2
        &= - \sum_{j=1}^p \sum_{i=1}^k \frac{\x_j \x_j^T \U \I_i}{\| \x_j \x_j^T - \U_i\U_i^T \x_j\|_2} - \bm{\Lambda}_2 \U\\
         \nabla_{\bm{\Lambda}_1} \mathcal{L}_1 &=  \nabla_{\bm{\Lambda}_2} \mathcal{L}_2 =  \I - \U^T \U,\\
    \end{aligned}
    \end{align*}

    Setting $\nabla_{\U} \mathcal{L}_1 = \bm{0}$, $\nabla_{\bm{\Lambda}_1} \mathcal{L}_1= \bm{0}$ and leveraging~\cref{eq: max_weights} to define $\{\W_i\}_i$ results in
    \begin{align*}
        \sum_{j=1}^p \sum_{i=1}^k \frac{\x_j \x_j^T \U \I_i}{\| \U_i^T \x_j\|_2} &=  \bm{\Lambda}_1 \U, \\
        \sum_{j=1}^p \sum_{i=1}^k \frac{\U^T \x_j \x_j^T \U \I_i}{\| \U_i^T \x_j\|_2} &=  \bm{\Lambda}_1, \\
        \sum_{j=1}^p \sum_{i=1}^k (\W_i)_{jj} \U^T \x_j \x_j^T \U \I_i &=  \bm{\Lambda}_1, \\
        \tr\left(\sum_{i=1}^k \U^T \left( \sum_{j=1}^p (\W_i)_{jj} \x_j \x_j^T \right)  \U \I_i\right) &=  \tr(\bm{\Lambda}_1), \\
        \sum_{i=1}^k \tr\left(\U^T \left( \sum_{j=1}^p (\W_i)_{jj} \x_j \x_j^T \right)  \U \I_i\right) &=  \tr(\bm{\Lambda}_1), \\
        h_{[\![ U]\!]}(\U) &=  \tr(\bm{\Lambda}_1).
    \end{align*}
        Similarly, setting $\nabla_{\U} \mathcal{L}_2 = \bm{0}$, $\nabla_{\bm{\Lambda}_2} \mathcal{L}_2= \bm{0}$ and leveraging~\cref{eq: min_weights} to define $\{\W_i\}_i$ results in
    \begin{align*}
        \sum_{j=1}^p \sum_{i=1}^k \frac{\x_j \x_j^T \U \I_i}{\| \x_j  - \U_i \U_i^T \x_j\|_2} &=  \bm{\Lambda}_2 \U, \\
        -\sum_{j=1}^p \sum_{i=1}^k \frac{\U^T \x_j \x_j^T \U \I_i}{\| \x_j  - \U_i \U_i^T \x_j\|_2} &=  \bm{\Lambda}_2, \\
        -\sum_{j=1}^p \sum_{i=1}^k (\W_i)_{jj} \U^T \x_j \x_j^T \U \I_i &=  \bm{\Lambda}_2, \\
        -\sum_{i=1}^k \tr(\U^T \left( \X \W_i \X^T \right)  \U \I_i) &=  \tr(\bm{\Lambda}_2),\\
        -h_{[\![ U]\!]}(\U) &=  \tr(\bm{\Lambda}_2).
    \end{align*}


% \begin{exmp}
% Suppose we sample points $\{\x^{(i)}\}_{i=1}^{5000} \subset \R^4$ with coordinates sampled as $\x^{(i)}_1, \x^{(i)}_2 \sim \mathcal{N}(0,1)$, $\x^{(i)}_3 \sim \mathcal{N}(0,0.5)$, and $\x^{(i)}_4 \sim \mathcal{N}(0,0.1)$ where $\mathcal{N}(\mu,\sigma)$ is a normal distribution with mean $\mu$ and standard deviation $\sigma$. \cref{fig:why_flag_pca1} emphasizes that the first two principal components of these data and the first two coordinates of these data are rotations of one another. \cref{fig:why_flag_pca2} shows nearly identical explained variance for the first two principal components and~\cref{fig:why_flag_pca3} shows the first two PCs are identically $0$ for the first two coordinates of the data. Overall, we should preform PCA on $\flag(2,3,4;5)$ instead of $\flag(1,2,3,4;5)$.
% \begin{figure}[H]
%     \centering
%     \includegraphics{figures/flag_exp_gaussian.pdf}
%     \caption{Mapping the data onto $\mathbf{e}_1 = [1,0,0,0]^T$ and $\mathbf{e}_1 = [0,1,0,0]^T$. Any basis vectors orthogonal to $\text{span}(\mathbf{e}_3, \mathbf{e}_4)$ will work for the first two principle components of our data.}
%     \label{fig:why_flag_pca0}
% \end{figure}

% \begin{figure}[H]
%     \centering
%     \includegraphics{figures/flag_exp_2pcs.pdf}
%     \caption{Mapping the data onto the first two principle components. Any basis vectors orthogonal to $\text{span}(\mathbf{e}_3, \mathbf{e}_4)$ will work for the first two principle components of our data.}
%     \label{fig:why_flag_pca1}
% \end{figure}

% \begin{figure}[t]
%   \centering
%   \subfloat{
%     \includegraphics[width=0.22\textwidth]{figures/flag_exp_gaussian.pdf}
%     % \label{fig:subfig1}
%   }
%   \hfill
%   \subfloat{
%     \includegraphics[width=0.22\textwidth]{figures/flag_exp_2pcs.pdf}
%     % \label{fig:subfig2}
%   }
%   \caption{Mapping the data onto $\mathbf{e}_1 = [1,0,0,0]^T$ and $\mathbf{e}_1 = [0,1,0,0]^T$ (left) and the first two principle components (right). Any basis vectors orthogonal to $\text{span}(\mathbf{e}_3, \mathbf{e}_4)$ will produce a rotated version of the same plots so in this case, PCA is not unique on $\flag(1,2,3;4)$.}
%   \label{fig:why_flag_pca1}
% \end{figure}


% \begin{figure}[t]
%     \centering
%     \includegraphics[width =\linewidth]{figures/flag_exp_evr.pdf}
%     \caption{The explained variances (objective function values) for the PCs. \tolga{These figures (7 and 8) are rather old and I am not sure which PCA-variants Example B.1 uses. If we want to integrate those, we have to adapt them to our new setting. If they don't mean much now, we can remove them.}}
%     \label{fig:why_flag_pca2}
% \end{figure}

% \begin{figure}[t]
%     \centering
%     \includegraphics[width =\linewidth]{figures/flag_exp_pcs.pdf}
%     \caption{The principal directions.}
%     \label{fig:why_flag_pca3}
% \end{figure}
% \end{exmp}


\begin{comment}
\begin{prop}\label{prop:IRLSPCA}
    Suppose $[\![\Y]\!] \in \flag(n+1)$ solves~\cref{eq: flagRPCAmax} and $\| \Y_i^T \x_j\|_2 \geq \epsilon$ for all $i$ and $j$. Then $\Y \in St(n_k,n)$ must also solve
    \begin{equation}\label{eq:STrealflagPCA}
        \argmax_{\Z \in St(n_k,n)} f_{[\![\Y]\!], \epsilon}(\Z) 
    \end{equation}
    where $\A$ is defined in~\cref{eq:A} using the appropriate weight matrix.
\end{prop}

\begin{proof}

    This allows us to rephrase the optimization problem in~\cref{eq:realflagPCA} as
    \begin{equation}
        \argmax_{\Y \in St(n_k,n)} \sum_{j=1}^p \sum_{i=1}^k \sqrt{\tr\left( \widetilde{\X} \mathbf{J}_j \widetilde{\X}^T \Y \I_i \Y \right)}.
    \end{equation}

    Now, we can write the Lagrangian for this problem with the symmetric matrix of Lagrange multipliers $\bm{\Lambda}$ as
    \begin{equation}
        \mathcal{L} (\Y) = \sum_{j=1}^p \sum_{i=1}^k \sqrt{\tr\left( \widetilde{\X} \mathbf{J}_j \widetilde{\X}^T \Y \I_i \Y \right)} + \bm{\Lambda}(\I - \Y^T \Y ).
    \end{equation}

    Then, we collect our gradients in the following equations
    \begin{align*}
    \begin{aligned}%\label{eq: lagrangian grad}
        \nabla_{\Y} \mathcal{L}
        &=  \sum_{j=1}^p \sum_{i=1}^k \frac{\widetilde{\X} \mathbf{J}_j \widetilde{\X}^T \Y \I_i}{\sqrt{\tr \left( \widetilde{\X} \mathbf{J}_j \widetilde{\X}^T \Y \I_i \Y \right)}} - \bm{\Lambda} \Y\\
         \nabla_{\bm{\Lambda}} \mathcal{L} &=  \I - \Y^T \Y.
    \end{aligned}
    \end{align*}

    \nate{finish}
    
\end{proof}


\begin{prop}
    Suppose $[\![\Y]\!] \in \flag(n+1)$ solves~\cref{eq: flagRPCAmin} and $\| \Y_i^T \x_j\|_2 \geq \epsilon$ for all $i$ and $j$. Then $\Y \in St(n_k,n)$ must also solve
    \begin{equation}\label{eq:STrealflagPCA}
        \argmin_{\Z \in St(n_k,n)} f_{[\![\Y]\!], \epsilon}(\Z) 
    \end{equation}
    where $f_{[\![\Y]\!], \epsilon}$ is defined in~\cref{eq: irls_f} and $\W_i$ is defined using~\cref{eq: min_weights}.
\end{prop}

\begin{prop}
    Suppose $[\![\Y]\!] \in \flag(n+1)$ solves~\cref{eq: flagDPCAmax} and $\| \Y_i^T \x_j\|_2 \geq \epsilon$ for all $i$ and $j$. Then $\Y \in St(n_k,n)$ must also solve
    \begin{equation}\label{eq:STrealflagPCA}
        \argmax_{\Z \in St(n_k,n)} f_{[\![\Y]\!], \epsilon}(\Z) 
    \end{equation}
    where $f_{[\![\Y]\!], \epsilon}$ is defined in~\cref{eq: irls_f} and $\W_i$ is defined using~\cref{eq: min_weights}.
\end{prop}

\begin{prop}
    Suppose $[\![\Y]\!] \in \flag(n+1)$ solves~\cref{eq: flagDPCAmin} and $\| \Y_i^T \x_j\|_2 \geq \epsilon$ for all $i$ and $j$. Then $\Y \in St(n_k,n)$ must also solve
    \begin{equation}\label{eq:STrealflagPCA}
        \argmin_{\Z \in St(n_k,n)} f_{[\![\Y]\!], \epsilon}(\Z) 
    \end{equation}
    where $f_{[\![\Y]\!], \epsilon}$ is defined in~\cref{eq: irls_f} and $\W_i$ is defined using~\cref{eq: min_weights}.
\end{prop}
\end{comment}
